# Supplementary material for: Generalized sparsity-promoting solvers for Bayesian inverse problems: Versatile sparsifying transforms and unknown noise variances
Source: arXiv:2402.16623 source file (2025-01-07)
Supplement: Supplementary file 1 [file convexity_supplement.tex]

% SIAM Supplemental File Template
\documentclass[review,supplement,onefignum,onetabnum]{siamonline220329}

\input{convexity_shared}

\externaldocument[][nocite]{ex_article}

% Optional PDF information
\ifpdf
\hypersetup{
  pdftitle={Supplementary Materials: An Example Article},
  pdfauthor={D. Doe, P. T. Frank, and J. E. Smith}
}
\fi

\begin{document}

\maketitle

\end{document}
